# Supplementary material for: ProtagonistTagger -- a Tool for Entity Linkage of Persons in Texts from Various Languages and Domains
Source: arXiv:2203.06746 source file (2022-03-13)
Supplement: Supplementary file 1 [file suplement.tex]

\documentclass[runningheads]{llncs}

\usepackage{graphicx}

\usepackage{times}
\usepackage{latexsym}

% For proper rendering and hyphenation of words containing Latin characters (including in bib files)
\usepackage[T1]{fontenc}
% For Vietnamese characters
% \usepackage[T5]{fontenc}
% See https://www.latex-project.org/help/documentation/encguide.pdf for other character sets

% This assumes your files are encoded as UTF8
\usepackage[utf8]{inputenc}

% This is not strictly necessary, and may be commented out,
% but it will improve the layout of the manuscript,
% and will typically save some space.
\usepackage{microtype}

\usepackage[linesnumbered,ruled,vlined]{algorithm2e}
\usepackage{graphicx}

\usepackage{url}

\begin{document}

\title{Supplement: \textit{ProtagonistTagger} -- a Tool for Entity Linkage of Persons in Texts from Various Languages and Domains}
\author{Weronika Łajewska\inst{1} \and Anna Wróblewska\inst{1}\orcidID{0000-0002-3407-7570} }

\authorrunning{W. Łajewska et al.}

\institute{Warsaw University of Technology, Poland \\
\email{weronikalajewska@gmail.com,anna.wroblewska1@pw.edu.pl}}

\maketitle   

In this supplementary material to our paper, we provide detailed analysis and statistics of our methods and datasets. This supplement contains the following sections:
\begin{itemize}
    \item the pseudo-code of the \textit{Matching Algorithm} procedure, along with a detailed description of each step (Section~\ref{appendix:matching_alg}),
    \item details about the performance of the NER models and the \emph{protagonistTagger}, as well as detailed statistics for specific novels (Section~\ref{appendix:statistics}),
    \item statistics for problems handled by the \textit{matching algorithm} (Section~\ref{stats_for_matching_alg_problems})
    \item an in-depth analysis of \textit{protagonistTagger} results --  detailed analysis of factors influencing the tool's performance (Section~\ref{appendix:results_analysis}),
    \item details for the experiments and the model reproducibility (Section~\ref{appendix:models_hyperparams}).
\end{itemize}

% !htb
\begin{algorithm*}[!ht]
\footnotesize
\SetAlgoLined
 potential\_matches = []\;
 \For{protagonist \textbf{in} protagonists}{
  ratio = regular\_string\_similarity(protagonist, named\_entity)\;
  \uIf{ratio == 100}{
   \textbf{return} match = protagonist\;
   }
  partial\_ratio = partial\_string\_similarity(protagonist, named\_entity)\;
  \uIf{partial\_ratio >= partial\_similarity\_precision}{
   potential\_matches\textbf{.add}(protagonist)\;
   }
  }
  potential\_matches = sorted(potential\_matches)  \# with respect to partial\_ratio \;
  match = \textbf{None} \;
  \uIf{len(potential\_matches) > 1}{
       match = potential\_matches[0]\;
       \uIf{prefix \textbf{is not None}}{
            \uIf{prefix == \emph{the}}{
            \textbf{return} match = \emph{the} + named\_entity}
            {
            title\_gender = get\_title\_gender(prefix) \# either female or male \;
             \For{potential\_match \textbf{in} potential\_matches}{
             \uIf{get\_name\_gender(potential\_match) == title\_gender}{
             \textbf{return} match = potential\_match}
             }
            }
       }
       \textbf{return} match
   }\uElseIf{len(potential\_matches) == 0}{
    original\_name = get\_name\_from\_diminutive(named\_entity)\;
    \uIf{original\_name \textbf{is not None}}{
    \textbf{return} match = protagonist from \emph{protagonists} that contains original\_name
    }
    \uElse{
    \textbf{return} "person"
   }
   }
   \textbf{return} potential\_match[0]
 \caption{Finding best match for the recognized named entity in the list of literary characters predefined for the analysed novel}
 \label{match_algorithm}
\end{algorithm*} 

\section{\textit{Matching Algorithm} Pseudocode}
\label{appendix:matching_alg}
The algorithm takes as inputs:
\begin{itemize}
    \item \textbf{named\_entity} -- a named entity of category \emph{person} found by NER model,
    \item \textbf{protagonists} -- a predefined list of all considered literary characters/protagonists,
    \item \textbf{prefix} -- a prefix that is a token appearing before the recognized named entity; it can be a personal title, the article \emph{the}, or an empty string,
    \item \textbf{partial\_similarity\_precision} -- value indicating how similar two strings need to be in order to be considered as potential matches; it is used as lower bound for \emph{partial string similarity} described in  the main paper.% in~Section~\ref{partial_string_matching}.
\end{itemize} \par

\subsection{Algorithm Analysis}
The first step of the \textit{matching algorithm} is to check (using \emph{regular\_string\_similarity}) if the \emph{named\_entity} is identical to any of the literary characters from the \emph{protagonists'} list (lines 3-5 in Algorithm~\ref{match_algorithm}). If so, the algorithm ends and returns it as the best match. However, if it is not the case, the \emph{partial\_ratio} is computed for the \emph{named\_entity} and each literary character from the protagonists' list using \emph{partial\_string\_similarity}. If it is above the given threshold (\emph{partial\_similarity\_precision}), a given name from the protagonists' list is considered as a potential match (see lines 6-8 in Algorithm~\ref{match_algorithm}). The list of potential matches is sorted decreasingly concerning the computed \emph{partial\_ratio} (line 10). \par

At this stage, the only thing left to do is check whether the considered named entity is one of the exceptions that we are handling. First of all, we check whether the prefix (token preceding the recognized named entity) can give us any clue (see lines 14-21 in Algorithm~\ref{match_algorithm}). If the prefix is:
\begin{itemize}
    \item the article \emph{the} -- the whole family with the surname given in the named entity is considered;
    \item one of the personal titles -- prefix's gender is recognized, then the first literary character from \emph{potential\_matches} list that has the same gender as the personal title in the prefix is returned (see lines 17-21 in Algorithm~\ref{match_algorithm}). Here, we need to assume that the name higher in the list is more probable due to the higher similarity score. It may not always be the case, but some simplifications are necessary. 
\end{itemize} 
The last considered variant appears when not even a single literary character was qualified as a potential match. The reason for such a situation may be that the named entity includes not the basic form of the name of the literary character but the diminutive. In such a case, the additional search is performed in an external dictionary of diminutives containing more than 3300 different forms of names (see lines 23-26 in Algorithm~\ref{match_algorithm}). If the named entity is not found in the diminutive dictionary, a general tag \emph{person} is returned. It means that any of the predefined tags match the named entity.

\section{Detailed Statistics of NER models' and \textit{ProtagonistTagger}'s Performance}
\label{appendix:statistics}

Our prepared testing sets for NER models (both, retrained and fine-tuned) comprises: \emph{Test\_large\_person} and \emph{Test\_small\_person}. These testing sets are manually annotated with general tag \emph{person} creating a gold standard for the NER model. The performance of \emph{protagonistTagger} is evaluated on \emph{Test\_large\_names} and \emph{Test\_small\_names}. Testing sets for \emph{protagonistTagger} include the same sentences as the corresponding sets used for testing the NER model. The only difference is that this time the sentences are manually annotated with full names of literary characters while creating the gold standard. \par

The performance of NER models (pretrained and fine-tuned) is evaluated on two testing sets: \emph{Test\_large\_person} and \emph{Test\_small\_person}. The overall performance of \emph{protagonistTagger} is evaluated on \emph{Test\_large\_names} and \emph{Test\_small\_names}.  \par

\begin{table*}
 \footnotesize
 \centering
 \setlength{\arrayrulewidth}{0.1mm}
\setlength{\tabcolsep}{3pt}
\renewcommand{\arraystretch}{1}
\begin{tabular}{ p{4cm}  p{1.5cm} | p{1.3cm}  p{1.3cm}  p{1.5cm}  p{1.3cm}}
%\hline
 \multicolumn{2}{c|}{\textbf{Novel title / NER model}} & \textbf{Precision} & \textbf{Recall} & \textbf{F-measure} & \textbf{Support} \\
\hline\hline
\multicolumn{6}{c}{\textbf{\emph{Test\_large\_person}}} \\
\hline\hline
The Picture of Dorian Gray
    & standard &  0.69 &  0.41 &  0.51 &  90 \\
    & fine-tuned &  0.74 &  1    &  0.85 &  90 \\
\hline
Frankenstein
    & standard &  0.91 &  0.62 &  0.74 &  93 \\
    & fine-tuned  &  0.78 &  0.98 &  0.87 &  93 \\
\hline
Treasure Island
    & standard &  0.75 &  0.66 &  0.7  &  97 \\
    & fine-tuned &  0.78 &  1    &   0.87 &   97 \\
\hline
Emma
    & standard &  0.84 &  0.77 &  0.81 &  115 \\
    & fine-tuned &  0.85 &  1    &  0.92 &  115 \\
\hline
Jane Eyre
    & standard &  0.86 &  0.78 &  0.82 &  97 \\
    & fine-tuned &  0.74 &  0.95 &  0.83 &  97 \\
\hline
Wuthering Heights
    & standard &  0.95 &  0.87 &  0.91 &  108 \\
    & fine-tuned &  0.88 &  0.99 &  0.93 &  108 \\
\hline
Pride and Prejudice
    & standard &  0.85 &  0.87 &  0.86 &  124 \\
    & fine-tuned &  0.8  &  0.98 &  0.88 &  124 \\
\hline
Dracula
    & standard &  0.86 &  0.94 &  0.9  &  97 \\
    & fine-tuned &  0.72 &  0.99 &  0.83 &  97 \\
\hline
Anne of Green Gables
    & standard &  0.91 &  0.96 &  0.94 &  114 \\
    & fine-tuned &  0.85 &  0.99 &  0.92 &  114 \\
\hline
Adventures of Huckleberry Finn
    & standard &  0.71 &  0.99 &  0.83 &  86 \\
    & fine-tuned &  0.61 &  1    &  0.75 &  86 \\
\hline
\textbf{-- Overall results --}
    & \textbf{standard} &  \textbf{0.84} &  \textbf{0.8}  &  \textbf{0.82} &  \textbf{1021} \\
    & \textbf{fine-tuned} &  \textbf{0.77} &  \textbf{0.99} &  \textbf{0.87} &  \textbf{1021} \\
\hline\hline
\multicolumn{6}{c}{\textbf{\emph{Test\_small\_person}}} \\
\hline\hline
The Catcher in the Rye
    & standard &  0.68 &  0.68 &  0.68 &  74  \\
    & fine-tuned &  0.58 &  0.91 &  0.71 &  74 \\
\hline
The Great Gatsby
    & standard &  0.75 &  0.84 &  0.79 &  102 \\
    & fine-tuned &  0.66 &  0.98 &  0.79 &  102 \\
\hline
The Secret Garden
    & standard &  0.9 &  0.82 &  0.86 &  97  \\
    & fine-tuned &  0.83  &  0.95 &  0.88 &  97 \\
\hline
\textbf{-- Overall results --}
    & \textbf{standard}  &  \textbf{0.78} &  \textbf{0.79} &  \textbf{0.78} &  \textbf{273} \\
    & \textbf{fine-tuned} &  \textbf{0.69} &  \textbf{0.95} &  \textbf{0.8}  &  \textbf{273} \\
\end{tabular}
\caption{Metrics computed for the standard NER model and the fine-tuned NER model for annotations with general label \emph{person}. The \emph{support} is the number of occurrences (mentions) of class \emph{person}.}
\label{tab:app:metrics_fine_tuned_ner}
\end{table*}

\begin{table*}
 \footnotesize
 \centering
 \setlength{\arrayrulewidth}{0.1mm}
\setlength{\tabcolsep}{3pt}
\renewcommand{\arraystretch}{1}
\begin{tabular}{ p{4cm}  p{1.5cm} p{1.5cm} p{1.5cm} }
%\hline
 \textbf{Novel title} & \textbf{Precision} & \textbf{Recall} & \textbf{F-measure} \\
\hline
\multicolumn{4}{c}{\textbf{\emph{Test\_large\_names}}} \\
\hline
Pride and Prejudice             &        0.84 &     0.85 &        0.83 \\
 The Picture of Dorian Gray     &        0.96 &     0.97 &        0.96 \\
 Anne of Green Gables           &        0.94 &     0.96 &        0.95 \\
 Wuthering Heights              &        0.79 &     0.77 &        0.77 \\
 Jane Eyre                      &        0.8  &     0.75 &        0.76 \\
 Frankenstein                   &        0.91 &     0.88 &        0.89 \\
 Treasure Island                &        0.92 &     0.91 &        0.91 \\
 Adventures of Huckleberry Finn &        0.89 &     0.93 &        0.9  \\
 Emma                           &        0.93 &     0.86 &        0.88 \\
 Dracula                        &        0.9  &     0.89 &        0.89 \\
\textbf{-- Overall results --}    &    \textbf{0.88} &     \textbf{0.87} &        \textbf{0.87} \\
\hline
\multicolumn{4}{c}{\textbf{\emph{Test\_small\_names}}} \\
\hline
 The Catcher in the Rye  &        0.8  &     0.77 &        0.78 \\
 The Great Gatsby        &        0.88 &     0.9  &        0.89 \\
 The Secret Garden       &        0.8  &     0.79 &        0.79 \\
\textbf{-- Overall results --}    &    \textbf{0.83} &     \textbf{0.83} &       \textbf{ 0.83} \\
\end{tabular}
\caption{Performance of the \emph{protagonistTagger}.}
\label{tab:app:full_tags_large_set_overall_metrics}
\end{table*}

The metrics for the performance of the NER model are presented in~Table~\ref{tab:app:metrics_fine_tuned_ner} and the performance of the whole \emph{protagonistTagger} tool is presented in~Table~\ref{tab:app:full_tags_large_set_overall_metrics}. All the metrics are given for each novel individually and for each testing set in general.

\section{Detailed Statistics for Problems Handled by the \textit{Matching Algorithm}}\label{stats_for_matching_alg_problems}
\subsection{Handling Diminutives of Literary Characters}
The most problematic cases in the matching process are diminutives and nicknames. The problem accompanies the character \emph{Elizabeth Bennet}, who is sometimes called \emph{Lizzy} by her family. Statistics presented in~Table~\ref{tab:Elizabeth} shows that in the case of \emph{Pride and Prejudice} by Jane Austen this problem is quite common. In order to discover a base form of a diminutive detected in a text, we use the external list containing the most common variants of names.  \par

\begin{table}
  \centering
  \footnotesize
    \begin{tabular}{ p{2.5cm}  p{2.5cm} }
        Named entity & \# of appearances \\ 
        \hline
         Elizabeth & 635 \\
         Lizzy & 96 \\ 
         Miss Bennet & 72 \\
         Miss Elizabeth & 12 \\ 
         Elizabeth Bennet & 8 \\ 
    \end{tabular}
    \caption{Appearances of the references to \emph{Elizabeth Bennet} in \emph{Pride and Prejudice} in different forms.}
    \label{tab:Elizabeth}
\end{table}

\subsection{Named Entities Preceded with Personal Title}
Another case that needs special consideration is a named entity consisting only of a surname. We consider this situation on the example of \emph{Bennet} named entity. As it is discussed in the paper, we want to distinguish between \emph{Bennet} meaning the whole family and \emph{Bennet} being the surname of a single character. We can do it by analyzing the word preceding the detected named entity. \emph{Bennet} preceded with a personal title such as Mr., Mrs., Ms. or Miss, should be identified as a single person, whose surname is \emph{Bennet}. In all other cases, \emph{Bennet} is treated as the whole family and not a single person identified in a text. The statistics presented in~Table~\ref{tab:Bennet} illustrates the scale of the problem in this specific novel, which has 121,533 words. The entity \emph{Bennet} appears 323 times, out of which 314 cases can be analyzed more precisely thanks to the preceding personal title.

\begin{table}
    \centering
    \footnotesize
    \begin{tabular}{ p{2.5cm}  p{2.5cm} }
        Named entity & \# of appearances \\
        \hline
         Bennet & 323 \\ 
         Mrs. Bennet & 153 \\ 
         Mr. Bennet & 89 \\ 
         Miss Bennet & 72 \\
    \end{tabular}
    \caption{Appearances of the named entity \emph{Bennet} in \emph{Pride and Prejudice} with different personal titles.}
    \label{tab:Bennet}
\end{table}

\section{\textit{ProtagonistTagger}'s Performance vs Number of Literary Characters}
\label{appendix:results_analysis}
One of the factors that intuitively should influence the performance of the \emph{protagonistTagger} is the number of literary characters in a novel that is analysed. The number of protagonists in a novel determines the number of tags that are used by the \emph{protagonistTagger}. The more tags the tool has to choose from, the more difficult is the task of matching them correctly to each recognized named entity. The relation between the precision of the \emph{protagonistTagger} and the number of tags per each novel is presented in~Figure~\ref{fig:names_amouts_graph}. It can not be said unambiguously that these two values are in inverse proportion in the analysed testing sets. The novels for which the tool achieved both the lowest and the highest precision -- \emph{The Picture of Dorian Gray} and \emph{The Secret Garden} -- have a relatively small number of literary characters. \par 

\begin{figure*}
    \centering
    \includegraphics[width=\textwidth]{Images/Number of tags per novel vs ProtagonistTagger precision (1).png}
    \caption{The left vertical axis describes the number of literary characters (tags used by the \emph{protagonistTagger}) in each novel, whereas the right vertical axis describes the precision of the \emph{protagonistTagger} (given in percents) for each novel. Novels used in \emph{Test\_small\_names} are marked with grey underlining.}
    \label{fig:names_amouts_graph}
\end{figure*}

Another factor that was suspected to negatively influence the performance of the \emph{protagonistTagger} is the number of tags sharing a common part. In the case of \emph{Bennet} family in \emph{Pride and Prejudice} by Jane Austen protagonists with the same surname are problematic even for human annotators. Sometimes a personal title preceding the named entity can be helpful. However, matching correctly tags that share the same surname or even name may be nontrivial. For that reason, we created statistics of tags that share some common part. These statistics, presented in~Table~\ref{tab:names_amounts}, are given for each novel included in both testing sets. Additionally, they are presented in~Figure~\ref{fig:names_common_parts_graph} along with the performance of the \emph{protagonistTagger}.

\begin{figure*}
    \centering
    \includegraphics[width=\textwidth]{Images/Percentage of tags with common part vs ProtagonistTagger precision (1).png}
    \caption{The right vertical axis describes the percentage of tags sharing a common part 
    (grey bars), as well as the precision of the \emph{protagonistTagger} (given in percents) for each novel in the testing sets. Novels used in \emph{Test\_small\_names} are marked with grey underlining.}
    \label{fig:names_common_parts_graph}
\end{figure*}

\begin{table*}
 \footnotesize
 \centering
 \setlength{\arrayrulewidth}{0.1mm}
\setlength{\tabcolsep}{3pt}
\renewcommand{\arraystretch}{1}
    \begin{tabular}{  p{5cm} | p{2cm} | p{2cm} | p{2cm}  }
    Title of the novel & \# literary characters/tags & \# tags that share a common part & \% tags that share a common part \\ [0.5ex]
    \hline
     Pride and Prejudice            & 18 & 13 & 72\% \\
     The Picture of Dorian Gray     &  9 &  4 & 44\% \\
     Anne of Green Gables           & 21 & 11 & 52\% \\
     Wuthering Heights              & 19 & 12 & 63\% \\
     Jane Eyre                      & 27 & 13 & 48\% \\
     Frankenstein                   & 19 &  4 & 21\% \\
     Treasure Island                & 17 &  4 & 23\% \\
     Adventures of Huckleberry Finn & 16 &  7 & 43\% \\
     Emma                           & 14 &  9 & 64\% \\
     Dracula                        &  9 &  2 & 22\% \\
     \hline
     The Catcher in the Rye         & 13 &  4 & 31\% \\
     The Great Gatsby               & 10 &  4 & 40\% \\
     The Secret Garden              & 10 &  7 & 70\% \\
    \end{tabular}
    \caption{The number of literary characters (tags used by \emph{protagonistTagger}) appearing in each novel and the number of tags that share a common part. A common part can be the same name or surname. The same personal title in two tags is not considered a common part.}
    \label{tab:names_amounts}
\end{table*}

\begin{table*}
 \footnotesize
 \centering
 \setlength{\arrayrulewidth}{0.1mm}
\setlength{\tabcolsep}{3pt}
\renewcommand{\arraystretch}{1}
    \begin{tabular}{  p{4cm} | p{8cm} }
    Parameter or component & Value and/or description \\ [0.5ex]
    \hline
    pretrained Spacy model & en\_core\_web\_sm (\url{https://spacy.io/models/en#en_core_web_sm})\\
        word features & Bloom word embeddings with sub word features \\
    pretrained model architecture & deep convolution neural network with residual connections \\
    fine-tuning iterations & 100 \\
    dropout rate & 0.5 \\
    batch normalization & minibatch (size - a series of compounding values starting at 4.0, stopping at 32.0, with compound equal to 1.001) \\
    optimizer & Adam (learning rate=0.001; beta1=0.9; beta2=0.999; eps=1e-08; L2=1e-6; grad\_clip=1.0; use\_averages=True; L2\_is\_weight\_decay=True) \\
    \end{tabular}
    \caption{Details about the pretrained NER model and parameters used for the fine-tuning procedure.}
    \label{tab:ner_params}
\end{table*}

However, again no obvious relation between these two values is visible. It may be caused by the fact that common parts in tags may not be related to the main protagonists (the ones that appear most often in the novel and the testing sets). Therefore, the testing sets are not representative enough in this case. For example, in the case of \emph{Anne of Green Gables} that has relatively many literary characters, half of which share the same name or surname, the tool's performance is very high. Nonetheless, in the case of \emph{Wuthering Heights}, with a similar number of protagonists, half of which again share a common name or surname, performance is much lower. It is caused by the fact that in \emph{Wuthering Heights} the tags that share common parts correspond to the main protagonists. Whereas, in the case of \emph{Anne of Green Gables} such common elements appear rather in tags corresponding to tangential characters. \par

In general, it can be concluded that the performance of the \emph{protagonistTagger} depends on many factors, not only the number of tags and the percentage of tags with the common part in a novel. These two factors, in some cases, can negatively influence the performance of the tool. However, this impact is not certain in the case of all novels.

\section{Details for Reproducing the Experiments}
\label{appendix:models_hyperparams}

The documented code along with the attached manual that is provided with this paper is the best starting point for reproducing experiments. The created scripts allow to repeat all the actions and run all the tests described in the paper. Annotated corpus of thirteen novels is provided as a part of the code. Nevertheless, it is possible to expand it with new annotated texts using the provided scrips (being a part of \textit{protagonistTagger}). Table~\ref{tab:ner_params} contains the summary of the parameters and techniques applied to fine-tune the pretrained NER model~\footnote{\footnotesize{\url{https://spacy.io/models/en\#en\_core\_web\_sm}}}. \par

The pretrained NER model uses embeddings with subwords features, convolutional layers with residual connections, layer normalization, and maxout non-linearity (its output is the max of a set of inputs) \cite{maxout}. The training data is shuffled and batched. For each batch, the model is updated with the training sentences from a batch. The dropout is applied as a regularisation technique to make it a little bit harder for the model to memorize data and reduce overfitting.

In order to successfully use scripts provided as a part of \emph{protagonistTagger} tool the following requirements need to be fulfilled:
\begin{itemize}
    \item Python 3.6
    \item PyYAML 5.3
    \item gensim 3.8
    \item numpy 1.18.2
    \item pytorch.transformers 1.2
    \item scikit-learn 0.22
    \item scipy 1.4.1
    \item spacy 2.2.4
\end{itemize}

Additionally the following external packages are used:
\begin{itemize}
    \item fuzzywuzzy 0.18~\footnote{\footnotesize{\url{https://pypi.org/project/fuzzywuzzy/}}}
    \item gender-guesser 0.4~\footnote{\footnotesize{\url{https://pypi.org/project/gender-guesser/}}}
    \item nickname-and-diminutive-names-lookup~\footnote{\footnotesize{\url{https://github.com/carltonnorthern/nickname-and-diminutive-names-lookup}}}
\end{itemize}

\bibliography{custom}
\bibliographystyle{acl_natbib}

\end{document}
